# Supplementary material for: Role of kinematic constraints in the time reversal symmetry breaking of a model active matter
Source: arXiv:2409.10425 source file (2024-09-16)
Supplement: Supplementary file 1 [file Supplementary_Information.pdf]

# Supporting Information for

## Role of kinematic constraints in the time reversal symmetry breaking of a model active matter

**Soumen Das, Shankar Ghosh, Tridib Sadhu, and Juliane U. Klamser**

**Juliane U. Klamser**
**E-mail: juliane.klamser@umontpellier.fr**

### This PDF file includes:

Figs. S1 to S3
Legends for Movies S1 to S4
SI References

### Other supporting materials for this manuscript include the following:

Movies S1 to S4

**Many-particle simulation.** Here, we provide details of the confining potential. Assuming that the center of the circular wall of radius $R$ is at the coordinate origin, the confining potential

$$U(R - r_i = r) = \begin{cases} 4\varepsilon\left[\left(\frac{\sigma/2}{r}\right)^{12} - \left(\frac{\sigma/2}{r}\right)^{6}\right] + \varepsilon, & \text{if } r < \frac{\sigma}{2}2^{1/6} \\ 0, & \text{otherwise} \end{cases}, \qquad [1]$$

where $\sigma$ is an indicator of the particle size, $\epsilon$ is the energy scale, and $\mathbf{r}_i = r_i(\cos\alpha_i, \sin\alpha_i)$ is the two-dimensional particle position.

**Materials.** The schematic of the mechanical assembly of the 'Squigglebot' made using SolidWorks is shown in Fig. S1. The moment of inertia of the assembly in the body frame can be calculated using SolidWorks as

$$J = \begin{pmatrix} 730.58 & 12.02 & -12.27 \\ 12.02 & 717.19 & 22.27 \\ -12.27 & 22.27 & 698.53 \end{pmatrix} \text{gm cm}^2 \qquad [2]$$

**Electronics:** A 6-axis accelerometer-gyroscope sensor module MPU6050 is placed inside the spheres to measure the instantaneous angular velocities which are then wirelessly transmitted by the wireless transceiver ESP-12E embedded in the microcontroller Wemos D1 mini. There is provision for wirelessly switching the motor on/off, thereby controlling the motion of the sphere. The current drawn from the battery is measured using a Hall effect based current sensor WCS2702 (1). The schematic diagram of the electronics circuit is shown in Fig. S2.

The micro-controller used for control, data collection and sensing is ESP-12F from Ai-Thinker Technology (2). It is an Wi-Fi enabled microchip based on ESP8266 SoC (System on Chip) module. ESP8266 integrates Tensilica's L106 Diamond series 32-bit RISC processor running at 80 MHz, 36 KB of RAM, 4 MB of external SPI flash, 10 bit ADC (analog to digital converter), I/O and a PCB-on-board antenna in the same chipThe module supports standard IEEE 802.11 b/g/n 2.4 GHz Wi-Fi and complete TCP/IP protocol stack. It also supports SDIO, SPI, $I^2C$, $I^2S$ and UART protocols for serial communication. The recommended power supply voltage for its operation is 3 - 3.7 V. Two decoupling capacitors of capacitance 0.1 $\mu$F (C5) and 10 $\mu$F (C6) are placed between the power supply (Vcc) pins and the ground close to the chip to filter out the high and low-frequency noise respectively. A push button switch is connected between the RST pin and ground for resetting the chip manually. RST, EN, GPIO0 and GPIO2 pins are connected to power supply VS via 10 k$\Omega$ pull-up resistors (R1, R2, R7, R6). GPIO15 is grounded via a 10 k$\Omega$ pull-down resistor (R5). GPIO0 pin needs to be shorted to ground temporarily to put it into the flash mode for uploading the code via UART protocol using an external programmer chip. ADC pin can handle a maximum voltage of 1 V. Since the output of the current sensor used for measuring the current drawn by the motor is more than 1 V, a voltage divider (consisting of resistors R3 and R4 - both 100 k$\Omega$) is used to decrease the input voltage to ADC pin. This sets the current resolution of the present experimental setup at 2.3 mA.

To measure the instantaneous angular velocity as well as the linear acceleration of the ball, MPU-6050 which is a MEMS based IMU (inertial measurement unit), is used (3, 4). MPU-6050 is an integrated 6-axis motion-tracking device that combines a 3-axis gyroscope, 3-axis accelerometer, and a Digital Motion Processor (DMP).

A MEMS accelerometer consists of a proof mass suspended on a spring. When the acceleration is applied on a particular axis, it causes the proof mass to shift to one side. Due to this deflection the capacitance between fixed plate and plate attached to the proof mass is changed. This change in capacitance is proportional to the acceleration. The sensor processes this change in capacitance and converts it into an analog output voltage (5). A MEMS gyroscope sensor is composed of a proof mass which is kept in a continuously oscillating motion. When a rotation is applied, the Coriolis force acting on the moving proof mass changes the direction of the vibration. This causes a capacitance change proportional to the angular velocity which is picked up by the sensing element and then converted to a voltage signal (5).

MPU6050 can measure the angular velocities with four programmable full scale ranges of $\pm250°$/s, $\pm500°$/s, $\pm1000°$/s and $\pm2000°$/s. Similarly it can measure the accelerations with full scale ranges of $\pm$2g, $\pm$4g, $\pm$8g and $\pm$16g, where g is the acceleration due to gravity. We use full scale ranges of $\pm2000°$/s and $\pm$2g for gyroscope and accelerometer respectively.

Following capacitors are used - (i) 0.1 $\mu$F regulator filter capacitor (C2) between REGOUT and ground, (ii) 0.01 $\mu$F bypass capacitor (C3) between VLOGIC and ground, (iii) 2.2 nF charge pump capacitor (C10) between CPOUT and ground and (iv) 0.1 $\mu$F bypass capacitor (C11) between power supply VDD and ground pins. $I^2C$ (6) is used for communication between MPU6050 and ESP-12F micro-controller. SCL is the $I^2C$ clock pin used to carry the timing signal supplied by the bus master device (ESP-12F). This pin is connected to the GPIO5 pin on ESP-12F. SDA is the $I^2C$ data pin used for both transmitting and receiving data. It is connected to the GPIO4 pin on ESP-12F. Both SCL and SDA pins are connected to the power supply voltage VS via two 4.7 k$\Omega$ pull-up resistors. The AD0 pin determines the $I^2C$ address of the module. This pin is connected to ground using a 4.7 k$\Omega$ pull-down resistor, which sets its $I^2C$ address as 0x68 in hexadecimal representation. Data is collected from MPU6050 at 25 Hz which is then transmitted over Wi-Fi by the micro-controller.

The maximum current that each GPIO pin of ESP8266 can supply is about 6 mA which is not sufficient to drive the motor. Hence, DRV8833 dual H-bridge motor driver is used to drive the motor (7). Another reason for using the motor driver is that without it, the noise from the motor can reset the control circuitry or burn out internal components of the micro-controller. The capacitors used are - (i) 10 $\mu$F ceramic bypass capacitor (C9) between the device power supply (VM) and ground pins, (ii) 0.01 $\mu$F X7R seramic capacitor (C4) between high-side gate driver VCP and VM pins and (iii) 2.2 $\mu$F bypass capacitor (C8)

between VINT and ground pins. AIN1 and AIN2 pins are connected to ground (Logic Low) and power supply VIN (Logic High) respectively. GPIO2 pin of ESP-12F is connected to NSLEEP (enable) pin of the motor driver. Therefore by setting the GPIO2 pin to logic High and Low, the motor driver and in turn the motor can be turned on and off.

Current drawn by the motor from the battery, is measured using a Hall effect based current sensor WCS2702 (1). The input power supply of the current sensor (VDD) is kept fixed at 3.3 V using LT1963A-3.3 linear and low-dropout (LDO) voltage regulator (8). The current resolution of the present experimental setup at 2.3 mA.

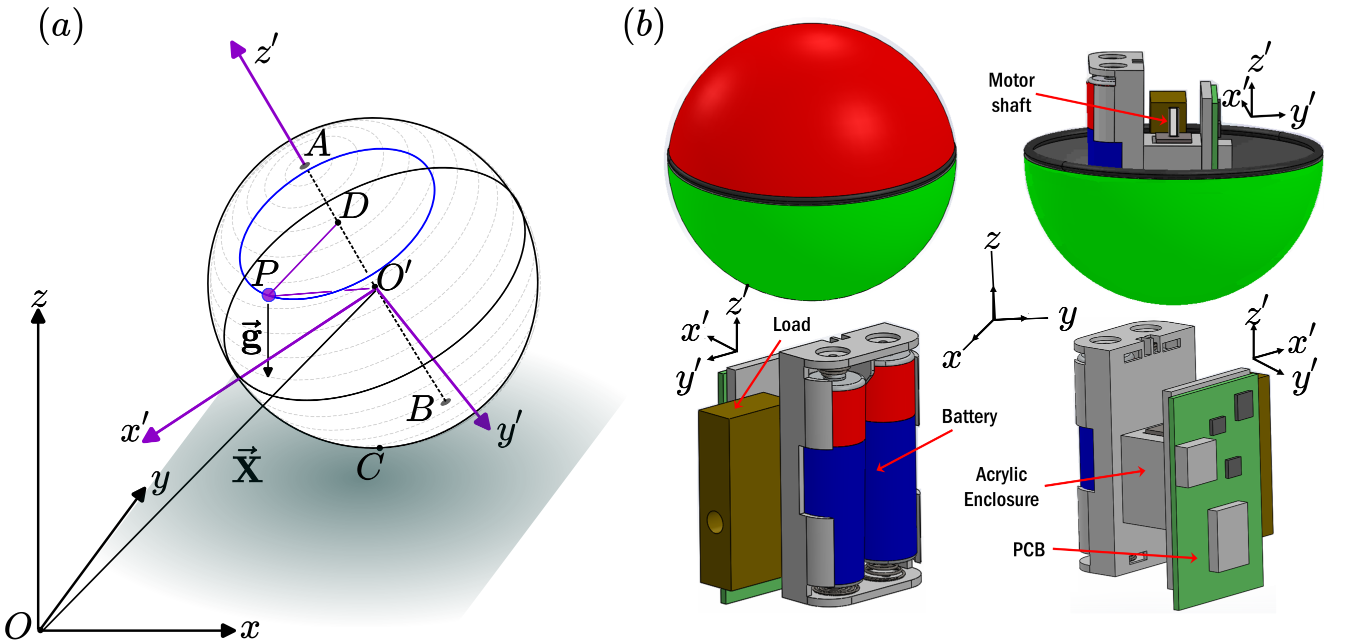


**Fig. S1.** (a) Schematic representation of the Squigglebot. The origin of the ball is at $O'$. The two relevant Cartesian frames are $\mathrm{O}'_{\mathrm{x}',\mathrm{y}',\mathrm{z}'}$ (fixed in space and in the body) and $\mathrm{O}'_{\mathrm{x},\mathrm{y},\mathrm{z}}$ (reference frame parallel to the lab-frame, but the origin at the center of the ball). Gravity points in the lab-frame along the $z$ axis. The direction of gravity is marked by down arrow in the figure. The position vector $\vec{X}$ describes the position of the point $O'$ with respect to the point $O$. (b) Schematic of the mechanical assembly with its different components pointed out. The convention of frames is same as in (a). The motor rotates about the body-y-axis.

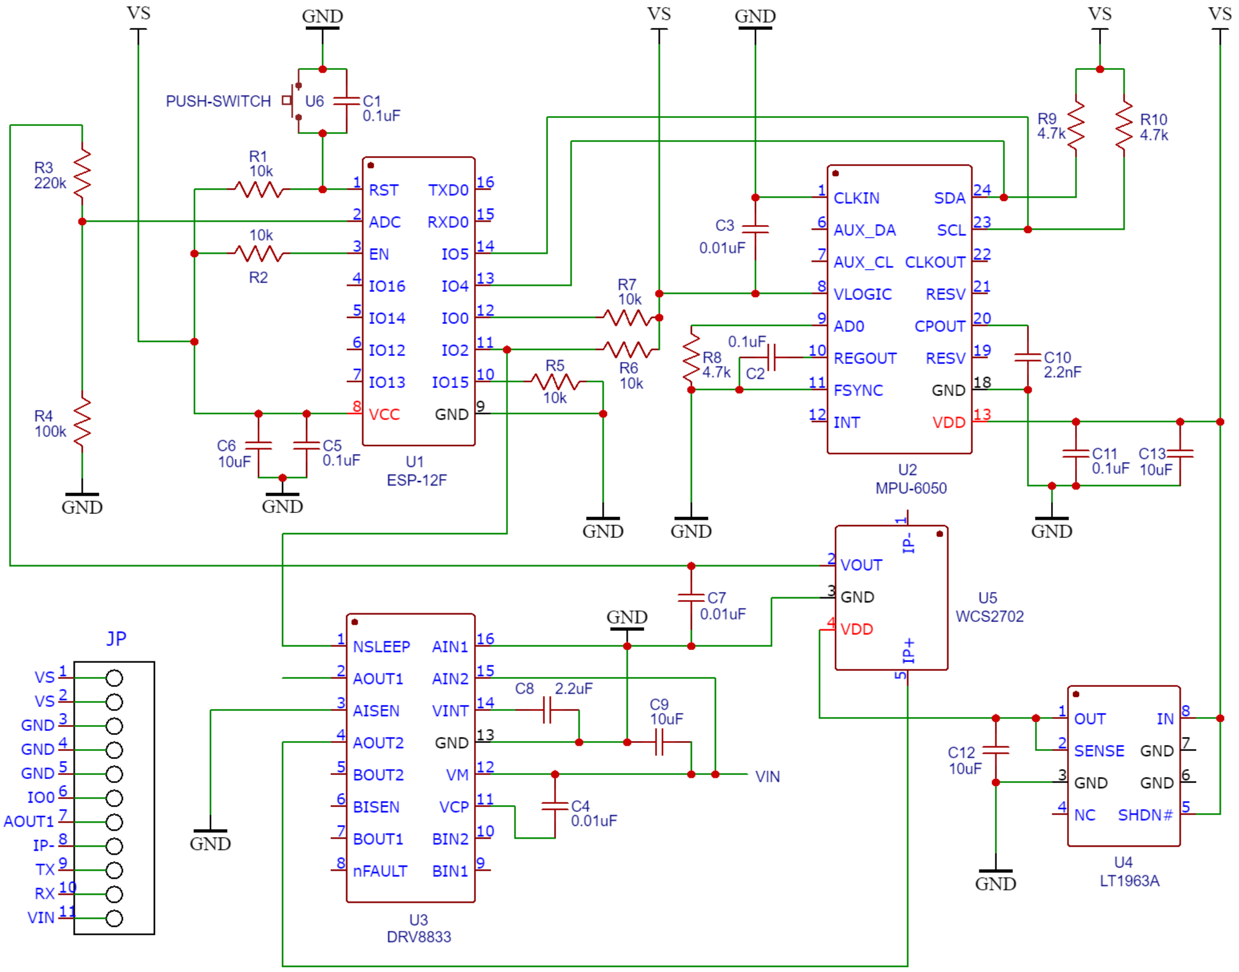


**Fig. S2.** Schematics of the circuit diagram used in the Squigglebot

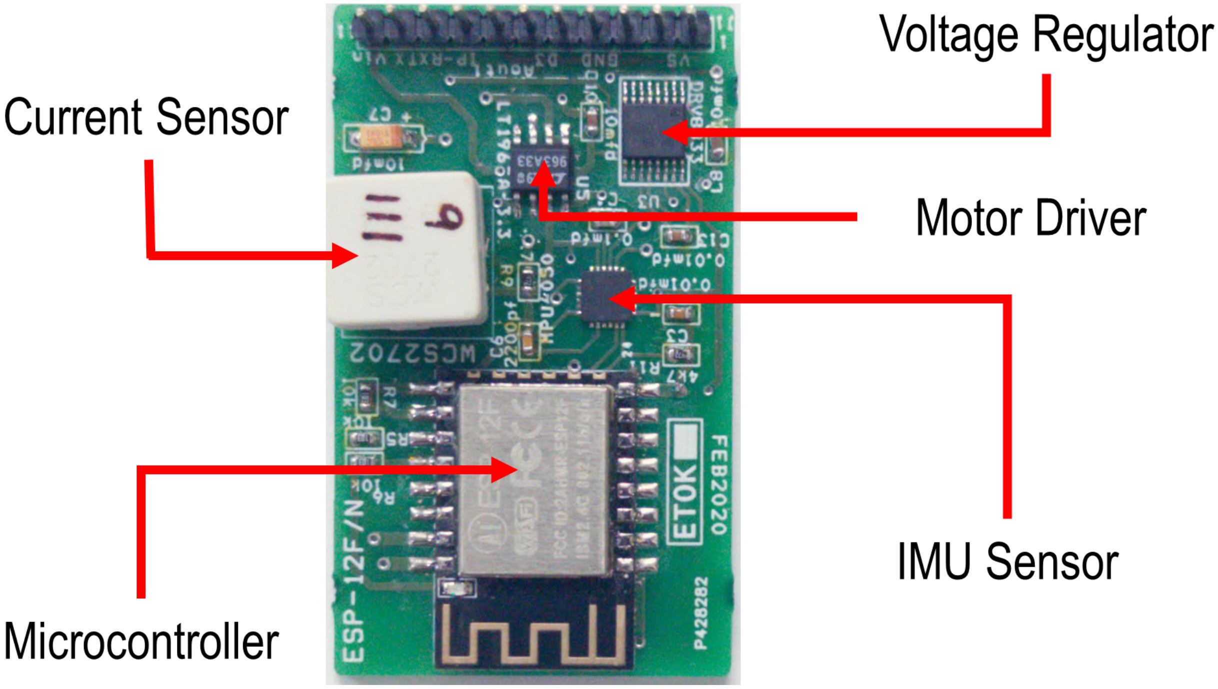


**Fig. S3.** Printed circuit board with the main components pointed out.

**Movie S1. Herding of passive balls by a single active Squigglebot. See movie at this link.**

**Movie S2. The dynamics of particle segregation for parameter values in Fig. 7b in the main text. See movie at this link.**

**Movie S3. The dynamics of herding for parameter values in Fig. 7c in the main text. See movie at this link.**

**Movie S4. The homogenized dynamics of particles for parameter values in Fig. 7d in the main text. See movie at this link.**

## References


1. Winson Semiconductor Corp., *WCS2702, Hall Effect Based Linear Current Sensor*, (2020).
2. Ai-Thinker Technology Co. Ltd, *ESP-12F Datasheet*, (2018) Rev. V1.
3. InvenSense Inc., *MPU-6000 and MPU-6050 Product Specification*, (2013) Rev. 3.4.
4. InvenSense Inc., *MPU-6000 and MPU-6050 Register Map and Descriptions*, (2013) Rev. 4.2.
5. S Nihtianov, A Luque, *Smart sensors and MEMS: Intelligent sensing devices and microsystems for industrial applications.* (Woodhead Publishing), (2018).
6. L Frenzel, Inter-Integrated Circuit (I2C) Bus in *Handbook of serial communications interfaces.* (Newnes), pp. 65–68 (2015).
7. Texas Instruments, *DRV8833 Dual H-Bridge Motor Driver*, (2015) Rev. E.
8. Linear Technology, *LTC1963A Series, 1.5A, Low Noise, Fast Transient Response LDO Regulators*, (2013) Rev. F.
